# Supplementary material for: Applying Interdisciplinary Frameworks to Understand Algorithmic Decision-Making
Source: arXiv:2305.16700 source file (2023-05-26)
Supplement: Supplementary file 1 [file supplemental_material.tex]

\section{Further details on the AMS algorithm}

\subsection{Development and public discourse}

The AMS algorithm incited heated public discourse over the benefits and risk of its deployment. According to the documentation accompanying its development \cite{Holl2018_Standards}, the algorithmic ranking should only be a suggestion to the employee at the Public Employment Agency, under the condition that the classified customer would be given a voice in the discussion about their employability. Further, discrepancies between algorithmic and human estimations of employability were meant to be reinserted into the algorithm to improve predictions, and finally, the classifications suggested by the algorithm were only to be used in this specific instance of customer support and in no other capacity. Additionally, the deployment followed three concrete overarching goals in the policy of the Employment Agency: a) increase in efficiency of consultation, b) increase in effectiveness of support measures, and c) standardisation of support measures and prevention of arbitrariness \cite{AMS_oeaw}.

However, the same technical documentation as cited above describes the risks of "problematic adaptation processes", including: over reliance on the statistical analysis, insufficient training of employees to overrule algorithmic suggestions, self-fulfilling prophecies of personal attributes that are controlled not by the individual but by their social environment, and pre-adjustment to the algorithmic suggestion by the customers in order to avoid bad classifications. In the document, transparency and ongoing scrutiny of the algorithm are listed as necessary measures to prevent these risks. Allhutter et al. further expanded on these points, listing additional severe risks of the algorithm's deployment \cite{AMS_oeaw}:

\begin{itemize}
    \item Reinforcement of societal biases due to reliance on historical data without adaptation to social change.
    \item Systemic discrimination due to the assignment of vulnerable groups to certain constellations.
    \item A shift from individual consultation to an overuse of computer-assisted decisions and automatising of interpersonal tasks. 
\end{itemize}

This detailed opposition to the deployment of an algorithmic decision-making system  by public institutions anticipates public discourse that could follow a large number of similar advances in the coming years. Due to the close examination of this specific project by the general public and its relatable domain, public job assignment and employment, the AMS algorithm represented a suitable example case for our analysis. We assessed that an understanding of the actual algorithm would provide a factual footing for the emotionally charged debate and a means for lay people to articulate their opinion precisely relating to specific components of the algorithm. For this reason, we used the AMS algorithm for a task-based qualitative study with the aim of engaging people in a detailed and nuanced discussion about the algorithm and its deployment.

\section{Initial introduction to the algorithm}

In the study, participants received a brief introduction to the algorithm after filling out the participant information form and the questionnaire, but prior to receiving an explanation variant (procedure depicted in \autoref{fig:procedure}).

This initial introduction contained a summary of relevant information about the algorithm and was intended to find out whether participants had a predetermined attitude or previous knowledge about the algorithm. The introduction contained the following information:

\begin{quote}
    The \amsalgorithm was commissioned and planned by the Public Employment Agency. Its goal was to predict job-seekers employability using their personal attributes such as age, gender, citizenship, education, and prior career. Depending on these attributes the algorithm of "high", "medium", or "low" chances of employment for the job-seeker, which was then confirmed or corrected by a human employee. The algorithm was piloted briefly but then put on hold due to concerns about data privacy. 
\end{quote}

After this introduction, participants were asked: "Do you think that you can at this point estimate what the consequences are of deploying such an algorithm in society?" Afterwards, participants proceeded to one of the three explanation variants.

\section{Questionnaire}

The full questionnaire that participants filled out in the beginning of the study is attached as a file in the supplementary material folder.

\section{Interview questions}

After completing both tasks, participants were asked several interview questions to learn more about their attitude towards the algorithm's deployment and their perceptions of algorithmic fairness, as well as to gather their feedback on the study. The following questions were asked:

\begin{enumerate}
    \item In your opinion, should the employee consult the algorithm for every job-seeker? Why?
    \item Suppose you were a job-seeker of the employment agency: Would you prefer that the employee of the employment agency would consult the algorithm on your case, or not?
    \item In each case, indicate on the scale which characteristic applies to the algorithm (Likert-scales from 1 to 7, 4 being neutral): (1) fair -- unfair (7), just -- unjust, legitimate -- illegitimate, social -- unsocial\footnote{Most of the studies were conducted in another language, where the adjective "social" has a slightly different meaning. It can be approximately translated as "serving the general public".}, biased -- unbiased and democratic -- undemocatric.
    \item In your estimation, what would a "fair" job placement system look like? What would it look like if it included the use of algorithms?
    \item How was your experience with the explanations? Did anything stand out to you? Did you miss anything in particular?
    \item What was your experience with the tasks? Did you find them easy or difficult to perform?
    \item Do you have any other comments or questions?
\end{enumerate}

\section{Explanation variants}

We designed three variants of the basic flowchart depicted in \autoref{fig:explanation}: textual, dialogue and interactive. Here we will give brief additional information on each variant. 

\subsection{Textual}

The textual variant consisted of the basic visual flowchart enriched by textual descriptions and some detail information, presented as a slideshow. Starting with a near blank slide, where only \textit{Hannah} was depicted, each new slide added another component to the flowchart and explained it with the aid of the descriptions. Two steps of this process are depicted in \autoref{fig:explanation_textual_1} and \autoref{fig:explanation_textual_2}. The participants could continue through the slides at their own pace and ask questions after finishing the explanation. 

\begin{figure}[h!]
    \centering
    \includegraphics[width=\textwidth]{images/Explanation_textual_1.PNG}
    \caption[Textual explanation 1]{Depiction of the resulting short-term employment chance for \textit{Hannah}, which is compared to the "standard group" in the textual explanation.}
    \label{fig:explanation_textual_1}
\end{figure}

\begin{figure}[h!]
    \centering
    \includegraphics[width=\textwidth]{images/Explanation_textual_2.PNG}
    \caption[Textual explanation 2]{Depiction of the group assignment using short-term and long-term employment chances in the textual explanation.}
    \label{fig:explanation_textual_2}
\end{figure}

\subsection{Dialogue}

The dialogue variant differed from the textual variant only in the fact that description were not presented textually but verbally from the study examiner. A protocol of the descriptions is added as a file in the supplementary material folder.

\subsection{Interactive}

The interactive variant was a simple web version of the basic flowchart, where buttons were added that when clicked would provide textual information. The full interactive version is depicted in \autoref{fig:explanation_interactive}, a covered version, as presented to the participants, is depicted in \autoref{fig:explanation_interactive_covered}. 

\begin{figure}[h!]
    \centering
    \includegraphics[width=\textwidth]{images/Explanation_interactive.PNG}
    \caption[Interactive explanation]{Depiction of whole flowchart in the interactive explanation. Three descriptions are expanded for demonstration.}
    \label{fig:explanation_interactive}
\end{figure}

\begin{figure}[h!]
    \centering
    \includegraphics[width=\textwidth]{images/Explanation_interactive_covered.PNG}
    \caption[Interactive explanation covered]{Areas of the interactive explanation are covered so as to avoid information overload. The covers vanished when clicked, as shown with the first cover.}
    \label{fig:explanation_interactive_covered}
\end{figure}

\section{Task section 1: \textit{Schifteh} and \textit{Harald}}

In the first task section, participants were consecutively presented with three sample cases of job-seekers: \textit{Martin}, \textit{Schifteh}, and \textit{Harald}\footnote{Example cases were taken from a detailed report on the \amsalgorithm \cite{AMS_oeaw}.}. \autoref{fig:martin_b} shows the first of these sample cases, \autoref{fig:schift_har} shows the last two. 

The procedure is depicted in \autoref{fig:martin_b}: Participants gave their subjective estimation of which measures could help the person to find work again (1), then gave their estimation of this person's chances for short-term and long-term employment\footnote{Short-term in the ASM algorithm is defined as being employed at least 90 days in the next seven months, long-term as at least six months in the next two years} (2), were then informed about the algorithmic scoring and the action taken by the employee (accepting or correcting the algorithm's decision plus any additional measures) and then indicated participants whether they perceived the algorithmic (3) and human (4) decisions as fair.

The three sample cases differed in their backstories, personal attributes as well as their algorithmic and human rankings. \textit{Martin} corresponds to the "standard group" of the algorithm: young men with compulsory education. Both algorithm and human assign him to group "medium". \textit{Schifteh} is a highly-skilled job-seeker who migrated to Austria and studied Computer Science. However, due to her nationality, gender, and missing data about her prior occupation, the algorithm assigns her to group "low". The employee upgrades her to group "medium", correcting the algorithm, and arranges a German course for her to participate in. \textit{Harald} is a waiter with a physical impairment who was unemployed for a longer time. In his case, both algorithm and employee assign him to group "low" and the employee does not provide him with measure for people 50+, despite his age of 49. 

\begin{figure}[h!]
    \centering
    \includegraphics[width=\textwidth]{images/Schifteh and Harald_anon.PNG}
    \caption[\textit{Schifteh} and \textit{Harald}]{\textbf{First task section}: Sample cases 2 and 3, \textit{Schifteh} and \textit{Harald}, each with short biographical description and personal attributes relevant for the algorithm. These cases were presented along with \textit{Martin} \autoref{fig:martin_b} in the first task section. Cases taken from Allhutter et al. \cite{AMS_oeaw}.}
    \label{fig:schift_har}
\end{figure}

\section{Task section 2: \textit{Sabine} and \textit{Michael}}

The second task section was split into two sub-tasks, depicted in \autoref{fig:sabine} and \autoref{fig:sabine_michael} respectively:\\
For the first sub-task (2.1), participants were provided with a sample case, (\textit{Sabine}), and were asked to explain to the study examiner how the algorithm would handle the case, in effect recalling the initial explanation (explanation depicted in \autoref{fig:explanation}, task depicted in \autoref{fig:sabine}).\\
In the second sub-task (2.2), participants received a case similar to the first one but ranked higher in terms of employability (\textit{Michael}). Participants should then indicate why \textit{Sabine} and \textit{Michael} were classified differently. The answer being that the first case was female and had duties of care, while the second was male and did not have duties of care (depicted in \autoref{fig:sabine_michael}).

\begin{figure}[H]
    \centering
    \includegraphics[width=\textwidth]{images/Sabine_anon.PNG}
    \caption[Second task section task 2.1]{\textbf{First subtask 2.1 in the second task section: explanation.} Participants should use the given information on the left to explain to the study examiner how the algorithm would come to a decision. The depicted questions were usually asked verbally and added here for clarity. Each question corresponds to a part of the explanation depicted in \autoref{fig:explanation}. \textit{Sabine} is assigned to group "medium" by the algorithm, the employee considers upgrading her to group "high".}
    \label{fig:sabine}
\end{figure}

\begin{figure}[H]
    \centering
    \includegraphics[width=\textwidth]{images/Sabine and Michael_anon.PNG}
    \caption[Second task section task 2.2]{\textbf{Second subtask 2.2 in the second task section: comparison.} Participants were asked to explain the algorithm using the profile of Sabine as an example in the first subtask (\autoref{fig:sabine}). In the second subtask (2.2), participants had to indicate why \textit{Sabine} and \textit{Michael} were classified differently despite largely similar profiles. The answer: \textit{Sabine}'s employability is ranked lower, as according to the algorithm women incur a loss of employability chance by their gender and another loss if they have duty of care for children or elderly. Additionally, the algorithm doesn't assign duty of care to men even if it they are a single parent, and can't take into account differences between full-time and part-time work.}
    \label{fig:sabine_michael}
\end{figure}

\section{Analysis and codes}

\subsection{Analysis}

For the analysis, we divided participants into three groups according to the explanation mode they were given: textual, dialogue, and interactive. Each group comprised ten participants (depicted in \autoref{fig:Participant_table}). Education levels were equal throughout the groups, but the second group had proportionally older participants, averaging 50 years, while group 1 averaged 33 and group 3 34 years. This can be traced to the fact that half of the studies in the second group were conducted in the local job employment agency, with both job-seekers and employees, who tended to be older than the regular café customer. 

To evaluate qualitative data we used an open coding approach, identifying and grouping key categories for each research question in the participants' responses. For an overview of the codes refer to \autoref{fig:codes}.

\textbf{Independent variables.} In the study, the independent variables consisted of the three explanation variants provided by us, the participants' previous knowledge about algorithm and the employment agency, their political attitude as well as their personal beliefs and experiences that contributed to their perceptions of algorithmic fairness.

\textbf{Dependent variables.} For \textbf{RQ1}, in which we asked how explanations would influence participants' understanding, we used three dependent variables: First, the self-reported understanding of the participants given once before and once after the task sections (as shown in \autoref{fig:procedure}). Second, the answers to the explanation task (2.1), and third, the answers to the comparison task (2.2).\footnote{For a description of tasks refer to Section~\ref{sec:tasks}}. Answers to questions 5 and 6 in the interview (Section~\ref{sec:procedure}) were used to further qualify the above measures. \\
Measuring understanding by letting participants explain the algorithm was motivated by studies which show that explaining newly learnt knowledge can support what Roscoe et al.~\cite{Roscoe2008} call \textit{reflective knowledge-building}: "to integrate new and prior knowledge and generate new ideas", while "[i]deas that are found to be incorrect or lacking may then be revised or reconstructed". We therefore used the explanation task to test participants' understanding of the explanation by comparing their descriptions with the major components of the flowchart and noting missing components.

For \textbf{RQ2}, relating to the factors that form perceptions of algorithmic fairness, we used the answers to the fairness assessments in the first task section (Section~\ref{sec:tasks}) and answers to the interview questions (Section~\ref{sec:procedure}) as dependent variables. By repeatedly prompting participants to provide their fairness estimation and inquiring why they chose this estimation in particular, we aimed to acquire a better understanding of which factors were most influential in building their fairness perceptions. 

For \textbf{RQ3}, regarding important factors for the acceptance of using algorithmic decision-making in the Public Employment Agency, we used answers to the interview questions 1 (use in society), 2 (use for self) and 4 (what is a fair job placement system) as dependent variables. After learning about the algorithm and the inclusion of human oversight, participants were expected to articulate which requirements in their view needed to be fulfilled in order to deploy the algorithm

\subsection{Codes}

Here we give a brief overview of the codes used. The codes \textit{understanding in terms of usage}, \textit{emotional engagement}, \textit{modifications}, and  \textit{limited understanding}, which were removed from the main text due to space constraints, are discussed in the next section.

\begin{figure}[H]
    \centering
    \includegraphics[width=\textwidth]{images/Codes_simple.PNG}
    \caption[Code structure]{Code structure for the qualitative analysis, split into \textit{understanding} and \textit{fairness}. \textit{Fairness} is further divided in three categories, partly inspired by Starke et al. \cite{StarkeChristopher2021}: algorithmic predictors, comparative effects and context of use.}
    \label{fig:codes}
\end{figure}

\section{Dimensions of understanding}

\subsection{Comparisons to own knowledge and experience}

We provide further quotes for the two codes \textit{comparisons to own knowledge} and \textit{comparisons to own experience}, described in Section~\ref{sec:findings}.

In terms of understanding, responses containing direct \textit{comparisons with the participants' own knowledge} were the most numerous theme of all, counting 129 mentions from 29 participants throughout the study. In these instances, participants relied on something they knew about algorithms, the employment agency or some other aspect of the study to incorporate the new information. One participant for example elaborated on the value of a master's degree from his perspective:  

\begin{quote}
    \textit{A master's is valuable, but there are few positions. And you're more likely to find a job in the long run, which you can then keep longer. Lower levels of education you can quickly use elsewhere, but it's unlikely anyone will hire a master's degree to do industrial cleaning.} (P12)
\end{quote}

Most participants used their previous knowledge to contextualise employment chances, comparing for example a job-seeker's personal attributes with what they knew about the demands of the job market. For some, this enabled them to question the algorithmic ranking by contrasting it with counterfactual information. One participant described this gap between algorithmic assessment and real world circumstances concerning the fact that men could not be assigned care obligations in the algorithm:

\begin{quote}
    \textit{That's why I was surprised about this last example [\textit{Michael} and \textit{Sabine}], because only the gender and the care obligations lead to this huge discrepancy, and I don't think that's appropriate. An employer has nothing to gain from having a person who is very well classified, but simply can't fulfil certain things because of care obligations [like \textit{Michael} has them]. He or she has to be somewhere at 5 o'clock at the latest to pick up the children.} (P13)
\end{quote}

The prevalence of this theme indicates that participants engaged with the information and integrated and compared it to their own knowledge, and thus understood it enough to perform this learning process. A closely connected category, \textit{comparisons with the participants' own experience}, counted 50 mentions from 22 participants. Here participants remembered something they had lived through while proceeding through the study, showing that some part of the information connected to their experience. For example, one participant anticipated the algorithmic decision in \textit{Schifteh's} case:  

\begin{quote}
    \textit{The algorithm will say group 'low'. She has no work experience. She has a good degree, but it’s not enough. I’m in the same situation so I relate it to myself.} (P21)
\end{quote}

In the sample case of \textit{Schifteh}, the agency's employee upgrades her and provides her with a German course (see section~\ref{sec:tasks}). The above response shows just how close the sample cases were to the participant's own experience. Employees from the local job agency confirmed this, stating that they practically met the fictive sample cases in their own work and could relate strongly to them. Another participant recalled her experience as a social worker, commenting on the sense of qualification measures:

\begin{quote}
    \textit{I worked for a long time in professional orientation with women in groups, and it is definitely the case that one pulls the other along. If a woman saw a friend going through training to become a home helper, she pulled along. "Then I'll do training, too." It was positive reinforcement.} (P18)
\end{quote}

\textit{Comparisons with own experience} show that participants did not only understand information, but also could connect and react to it emotionally, which is closely connected to the next theme, \textit{emotional engagement}. 

\subsection{Emotional engagement}

\textit{Emotional engagement} captures statements of participants who reacted to decisions that they perceived to be unfair in an emotional way, questioning for example the choices of attributes in the algorithm or the human decision of confirming a bad ranking. The character of statements varied, ranging from amused comments, over sympathy with the sample cases, to detailed criticism and general remarks about the system. These forms of emotional engagement suggest that participants understood some part of the algorithm enough to form an opinion about it and articulate it with emphasis, simultaneously showing that the topic was charged for them. In total, 64 statements from 25 participants included some form of emotional response, listed in \autoref{fig:emotional_engagement_table} in the supplementary material. 

As a side note, for a small group of participants the study also allowed for a shift in perspective:
\begin{quote}
    \textit{I found it difficult and I felt that I had to approach it psychologically, I had to put myself in people's shoes and in the end people are much more complex. Something like mental health, for example, is not considered at all.} (P3)
\end{quote}

As these citations show, people reacted strongly to the topic, especially when they considered the algorithmic or human decision to disadvantage someone.

\begin{table}[H]
\caption{Responses categorised as \textit{emotional engagement}, grouped in four subcategories.}
\centering
\scalebox{0.9}{%
\begin{tabular}{|p{3cm}|p{3.4cm}|p{3.4cm}|p{5cm}|}
\hline
Amused comments & Sympathising with sample cases & Detailed criticism & General remarks about the system \\ \hline
Aha,   funny, then the algorithm really is a stupid sexist! (P28)
& {[}Relating to Harald{]} I do find it a bit unfair that he doesn't get measures for people 50+. He's 49, how close to 50? Two more months and then he gets it?   Some goodwill would be appropriate. (P10) 
& {[}Comparison between Sabine and Michael{]} The only thing that speaks for him is gender, that accounts for 10\% better chances. That's pretty hefty. (P13) 
& I don't know why all this is   going in this direction now. It didn't exist 20 years ago and the world   worked just as fine, 100 years ago too. (P17)
\\ \hline
Okay,   so the standard group has 52\%, \textit{Hannah} has 42\%. And that's in central   Europe! That should be the same. (P20) 
& {[}Relating to Schifteh{]} That's hard, if it says 22\% and she has a master's degree,   also compared to example 1 (Martin).
& Do women automatically get lower scores? Well, where does discrimination start, where does it end? (P15)
& It all comes from a neoliberal   interest; we were always told as children under socialism what you can and   can't, should and shouldn't become; now we have free capitalism, it tells us   the same thing. It's just as fucked up. A different ideology, but the free   development of the human being is no longer even put forward as an idea. (P8) 
\\ \hline
\end{tabular}}
\label{fig:emotional_engagement_table}
\end{table}

\subsection{Understanding in terms of usage}

This category is a middle ground between \textit{bigger picture} and \textit{detail}, as it captured every mention of how the algorithm could be used as a tool to facilitate the tasks of the agency's employees. The frequency of this category (98 mentions from 29 participants) shows that participants were often able to take the perspective of the agency's employee, considering from how the algorithm's usage could affect their working practice. For us, this represents a part of what DeVito et al. \cite{devito2018} call "folk theories": perceiving the presented information through the lenses of lay people, including the shifts in perspectives that they themselves undertake.

This theme shows a form of pragmatical understanding, answering for example the question: How would this algorithm be used in the actual employment agency? One participant stated:
\begin{quote}
    \textit{Yes, the algorithm can be used, but only if there is a conversation with the supervisor. As a second opinion to complement the personal opinion, but not as a 100\% decision.} (P8)
\end{quote}

Interestingly, some participants questioned a decision made solely by a human, assigning it a kind of random quality, and valued the algorithmic decision in comparison. This perception of "algorithmic objectivity" is also discussed in the Section~\ref{sec:rq2}. One participant elaborated on the value of the algorithm as a second advice:

\begin{quote}
    \textit{So I don't think it's a bad thing if both algorithm and human make a decision. I wouldn't rely on either alone. Even if it would be a purely human decision, I would also like to have two consultants, two opinions, that can be extended by an algorithm for all I care.} (P12)
\end{quote}

Participants further related to the algorithm's usage by asking whether employers would know about the ranking, making comparisons to scoring systems in other countries, or by emphasising the value of human work:

\begin{quote}
    \textit{The consultation that we do with people over a longer period of time, over three months -- they think they can simulate this through a program. This blurs the assessment to the power of 100, but of course it is fast and inexpensive.} (P18)
\end{quote}

This shows that participants thought about the advantages and disadvantages of algorithmic decision-making, considering what ADM would mean in their own case. 

\subsection{Modifications}

In contrast to \textit{bigger picture}, \textit{detail} shows understanding on a fine-grained level, requiring a more in-depth comprehension of the concrete algorithmic workings. A continuation of this topic are suggestions to modify or change some aspects about the algorithm: \textit{modifications to the algorithm}. The theme counted 19 mentions from 15 participants and often included suggestions to change or exclude features in order to adapt the algorithm better to reality:
\begin{quote}
    I\textit{ think the classification is quite rough for a far-reaching decision. There are not too many criteria and others of relevance are not included -- like the driver's license. And I also find it odd that there are only three groups; if you had five groups, you might be more flexible.} (P13)
\end{quote}

Many participants used the topic of gender inequality to propose changes, making it a condition for the theoretical deployment of the algorithm. One participant noted:

\begin{quote}
    \textit{The gender inequality has to be changed, you have to see what is the reason for that and you have to change that. That's not how that should be used. 10\% less -- women have a disadvantage compared to men.} (P20)
\end{quote}

The ability to suggest \textit{modifications} of the algorithms points to a rather nuanced understanding, as it not only requires comprehension of the relevant components, but also the imagination to draw up other solutions and an awareness of the underlying problem. One participant for example commented on the use of the variable "regional labour market":

\begin{quote}
    \textit{This regional job market was too vague for me, you definitely need a differentiation of job fields which could include information like language skills and how important it is that you speak a certain language.} (P28)
\end{quote}

For a future study, exploring propositions to change the algorithm could be a promising avenue of research. Dietvorst et al.'s \cite{dietvorst2016} findings also suggest that algorithm aversion decreases if participants can only slightly modify the respective algorithm.

\subsection{Limited understanding}

\textit{Limited understanding} of the algorithm counted 27 mentions from 12 participants, significantly less than the previous categories. Often, incomprehension related to confusion about the meaning of a feature or another technical question. One participant stated that he couldn't assess what the percentages meant in short-term and long-term employability: 
\begin{quote}
    \textit{When you say the algorithm is at 23\%, that's 40\% less than 66\%, but how much is that? I find that difficult to assess.} (P9)
\end{quote}

Notable were difficulties in explaining the algorithm in subtask 2.1, which was the point were most of the \textit{limited understanding} mentions occurred. Some participants could not articulate what they wanted to say, either pointing to the abstract nature of the algorithm or missing information:

\begin{quote}
    \textit{The thing with the conversion I did not understand, I do not know the formula. Otherwise, I have halfway understood it, the data is simply used to ... I do not know how to explain it.} (P9)
\end{quote}

This challenges in reproducing learnt information -- encountered in lesser forms by most of the participants -- shows that understanding of this particular information is not complete, either as the words or the concepts are not known. Of course, conducting a task-based study meant that the study examiner involuntarily put  participants through a form of examination, which might hamper articulation or memorisation.
